# Supplementary material for: Laser-Ion Lens and Accelerator
Source: arXiv:1908.11768 ancillary file (2020-11-17)
Supplement: Supplementary file 1 [file Ion_Target_Final_Supp.pdf]

# Laser-Ion Lens and Accelerator: Supplemental Material

Tianhong Wang[1], Vladimir Khudik[1,2], and Gennady Shvets[1]
[1] *School of Applied and Engineering Physics, Cornell University, Ithaca, New York 14850, USA.*
[2] *Department of Physics and Institute for Fusion Studies, The University of Texas at Austin, Austin, Texas 78712, USA.*
(Dated: April 28, 2020)

## I. DIMENSIONAL ANALYSIS OF DM EQUATIONS IN TWO LIMITS

In this Section, we analyze the simplified Deformable Mirror (DM) equations. Dimensional analysis is then used to derive simple scalings of the target focal length $L_f$ and the ion momentum $p_x$ at the focal point. Two limiting cases are considered below: (i) large dimensionless acceleration ($\Gamma \gg 1$) resulting in a relativistic momentum $p_x \gg m_i c$, and (ii) small dimensionless acceleration ($\Gamma \ll 1$) resulting in a sub-relativistic momentum $p_x \ll m_i c$.

First, we consider the case (i) corresponding to large target acceleration and relativistic motion. In this regime, the target bending is insignificant: $\alpha_i \approx 0$, $\phi \approx 0$, and $\alpha_i'' \ll |d''| = 1$, $\phi'' \ll |d''| = 1$. See Fig.1 and the main text for the definition of these geometric parameters. Here $'$ stands for a derivative with respect to $r_0$. The DM equation derived from Eq. (4) under these assumptions takes the following form:

$$\dot{p}_r = -\frac{\Gamma}{d}\frac{1-\beta}{1+\beta}\frac{r}{r_0}x', \quad \dot{p}_x = \frac{\Gamma}{d}\frac{1-\beta}{1+\beta}\frac{r}{r_0}r', \tag{S1}$$

where 'over-dot' denotes the time derivative and $d = 1 - r_0^2/2$. Since $p_x \gg 1$, we can approximate $\gamma \approx p_x$, $p_r \approx p_x \dot{r}$ and $(1-\beta)/(1+\beta) \approx 1/4p_x^2$. For an arbitrary target element, we can also approximate the contraction of the target by introducing a transverse contraction coefficient $\chi(t)$ such that $r(t, r_0) = \chi(t) r_0$. We refer to this simplified description as the uniform contraction (UC) model, and show below that $\chi(t)$ vanishes at the focal point of the target.

The Eqs. (S1) then transform to:

$$\frac{4p_x^2}{\chi}\frac{\partial}{\partial t}(p_x\dot{\chi})r_0 = -\frac{\Gamma}{d}x', \tag{S2}$$

$$\frac{4p_x^2}{\chi^2}\dot{p}_x = \frac{\Gamma}{d}. \tag{S3}$$

Since the transverse motion of all target elements can be describable by the same $\chi(t)$, we can just concentrate on the target elements near the axis: $d \simeq 1$ for $r_0 \ll 1$. Take the derivative of Eq. (S2) respect to $t$, we get the following equation for $\chi$:

$$\frac{\partial}{\partial t}\Big[\frac{4p_x^2}{\chi}\frac{\partial}{\partial t}(p_x\dot{\chi})\Big]r_0 = -\Gamma v_x'. \tag{S4}$$

Bending of the target is caused by the variation of longitudinal velocity $v_x$ along the target radius which follows from the variation of the target thickness. Taking a derivative of Eq. (S3) with respect to $r_0$ and using the relationship $\dot{x}' \approx p_x'/p_x^3$, we find after additional algebraic transformations that

$$\frac{\partial}{\partial t}(4p_x^5 v_x') = r_0 \Gamma \chi^2. \tag{S5}$$

In the UC model, we assume the target moves as a whole: $p_x(r_0, t) \simeq p_x(0, t)$ for any $r_0$. Without changing the notations, the $p_x$ and $v_x'$ in equations (S4) and (S5) now refer to the $p_x(t)$ and $v_x'(t)$ which are independent of $r_0$. Therefore equations (S4) and (S5) are now only linear functions of $r_0$. Moreover, in the linearizing process of Eq. (S3) we have taken advantage of the parabolic dependence of $d(r_0)$: the derivative of the 'acceleration' $\Gamma/d(r_0)$ along $r_0$ must be linear in order to balance the variation of longitudinal velocity $v_x$.

Now with the same assumption: $d \approx 1$ and $p_x \equiv p_x(t)$, we can change our notation from $\partial/\partial t$ to $d/dt$ and transfer Eq. (S3) to the equation of motion of the target as a whole:

$$4p_x^2 \frac{d}{dt}p_x = \Gamma\chi^2. \tag{S6}$$

It follows from Eqs. (S5) and (S6) that $v_x' = r_0/3p_x^2$. This reduces Eq. (S4) to

$$\frac{d}{dt}\left[\frac{4p_x^2}{\chi}\frac{d}{dt}(p_x\dot{\chi})\right] = -\frac{\Gamma}{3p_x^2}. \tag{S7}$$

We have reduced the UC model to a set of two ordinary differential equations (ODEs): Eq. (S6) for the longitudinal momentum $p_x(t)$ and Eq. (S7) for the transverse contraction coefficient $\chi(t)$. The key assumption behind this derivation is that we can neglect the dependence of $p_x$ on $r_0$ and assume that $p_x \equiv p_x(t)$ in the $\Gamma \gg 1$ case. This is indeed confirmed by Fig. S1, where Figure S1 (a) shows the focusing of target at $\Gamma = 10$, and the black curves in Fig. S1 (b,c) represent the overlapping trajectories $\chi(t)$ and $p_x(t)$ of every target element. Each trajectory corresponds to a target element starting with different $r_0$ at $t = 0$. The red lines in Figs. S1 (b) and (c), respectively, show the $\chi(t)$ and $p_x(t)$ obtained from the UC model defined by the Eqs. (S6, S7); they agree with the DM model quite well. The only discrepancy appears in Fig. S1 (b): the solution of $\chi(t)$ somewhat deviates from the DM model because of our assumption that $\alpha_i \approx 0$ in Eqs. (S1). By ignoring the light incident angle $\alpha_i$, we assume the laser pressure is always applied normally to the target surface. That is why our $\chi(t)$ solution reaches the focal point earlier than the more accurate prediction of the DM model. In fact, even a small angle $\alpha_i$ may become comparable with $(1-\beta)$ at the later stage of target acceleration and focusing.

Finally, in Fig. S1 (d) we compare the solution from Eq. (S6) and Eq. (S7) with the $\chi(t)$ extracted from a full-PIC simulation. 200 different target elements are selected from the simulation in Fig. 3 of the main text and their trajectories $r/r_0$ are plotted as blue curves. The trajectories exhibit a considerable spread because of the more complete physics included in a full-PIC simulation. However, they are still in reasonable agreement with the UC model solution.

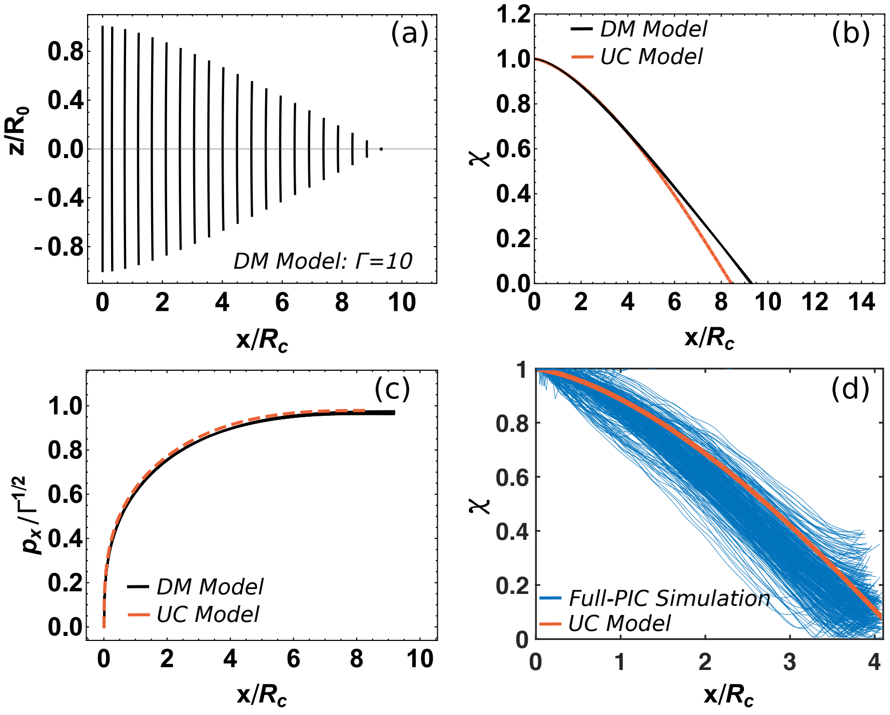


FIG. S1: Comparison between the solutions of the full Deformable Mirror(DM) and the reduced Uniform Compression (UC) models for $\Gamma = 10$. (a) DM model: insignificant target bending; the focusing is well described in the paraxial approximation. The contraction function $\chi(t)$ (b) and the target momentum $p_x$ (c) from the DM (black lines) and UC (red line) models. The black thick lines in (b) and (c) represent groups of trajectories with different starting $r_0$. (d) Blue trajectories: $\chi = r/r_0$ extracted from a full-PIC simulation with $\Gamma = 1.6$ (see Fig. 3 of main text), each curve represents one target element. Red curve: $\chi(t)$ from the UC model. The UC model is defined by Eqs. (S6, S7).

One can exclude $\Gamma$ from Eqs. (S6, S7) by introducing new variables $\tilde{p}_x = p_x/\Gamma^{1/2}$ and $\tilde{t} = t/\Gamma^{1/2}$. Therefore, $p_x \propto \Gamma^{1/2}$ and $ct \sim x \propto \Gamma^{1/2}$. Rigorous analysis of Eqs. (S1) leads to the scaling of momentum at $\Gamma > 1$: $p_x \approx \Gamma^{1/2}$, and the following scaling formula that is valid for both small and large values of $\Gamma$: $L_f \approx \left(2\Gamma^{1/2} + 2.95\right) R_c$.

The case (ii) is less dramatic because of its low acceleration and sub-relativistic final target energy. However, it is easier to realize using present-day laser systems. In this limit, the target undergoes significant bending while moving

with sub-relativistic speed. Therefore, after neglecting the $\beta$ and $|\vec{p}|^2$ terms in Eqs. (4,5), respectively, we can exclude the acceleration parameter $\Gamma$ from the DM equations Eq. (5):

$$\frac{\partial^2 \vec{r}}{\partial \tilde{t}^2} = \frac{\cos^2 \alpha_i}{d(r_0)} \frac{r}{r_0} (r' \vec{e}_x - x' \vec{e}_r), \tag{S8}$$

where $\tilde{t} = t\Gamma^{1/2}$ is the normalized time. Eq. (S8) can be easily solved numerically and its solution is shown in Fig. S2 for the thickness distribution $d(r_0) = 1 - r_0^2/2$. The black curve in Fig. S2 (a) shows the $r/r_0$ as a function of propagation distance for each target element, therefore the black curve represents a group of multiple trajectories. Different trajectories are overlapped that implies the uniform compression of the target. Trajectories cross $r = 0$ at the same value of $x$, and we find that the focal length is $L_f = 2.95R_c$, which is independent of $\Gamma$. In Fig. S2 (b), the momentums of different target elements are also represented by a group of multiple trajectories, the noticeable spread is due the velocity variation which follows from the thickness variation. As shown in Fig. 2 (a) of main text, this variation across different elements results in a significant bending of the target during acceleration. At the focal point, the target momentum is $p_x \approx 1.6\Gamma^{1/2}$ in this (sub-relativistic) limit.

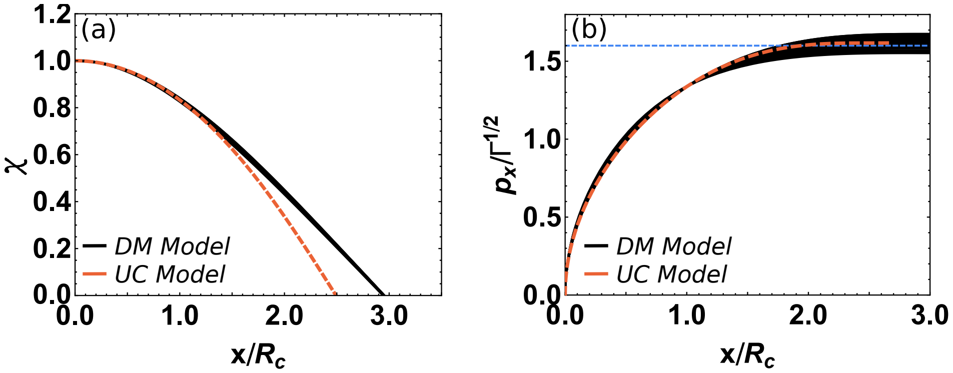


FIG. S2: Comparison between the solutions of the full Deformable Mirror(DM) and the reduced Uniform Compression (UC) models for $\Gamma \ll 1$. The contraction function $\chi(t)$ (a) and the target momentum $p_x$ (b) from the DM (black lines) and UC (red line) models. The black thick lines in (a) and (b) represent groups of trajectories with different starting $r_0$. The UC model is defined by Eq. (S13).

Figure S2 (a) implies we can use the same approach as in case (i), by assuming an universal solution of $\chi(t)$ for all target elements. One simple and less rigorous approximation is to assume $\cos^2 \alpha_i \approx 1$ in Eq. (S8) (this approximation would increase the radiation pressure normal to the target surface and result in faster focusing, however it would not change the property of Eq. (S8)). Replacing $r/r0$ and $r'$ by $\chi(t)$, we then transform Eq. (S8) to:

$$\frac{\partial^2 x}{\partial t^2} = \frac{\chi^2(t)}{1 - r_0^2/2}, \tag{S9}$$

$$r_0 \frac{\partial^2 \chi(t)}{\partial t^2} = -\frac{\chi(t)}{1 - r_0^2/2} \frac{\partial x}{\partial r_0}. \tag{S10}$$

Taking the $\partial/\partial r_0$ derivative of Eq. (S9) and assuming that the target element is near the axis ($r_0 \ll 1$), we obtain:

$$\frac{\partial^3 x}{\partial t^2 \partial r_0} = r_0 \chi^2(t). \tag{S11}$$

Neglect the $r_0^2$ term in Eq. (S10) and plug Eq. (S11) into Eq. (S10), we derive the following equation for $\chi(t)$ :

$$\frac{d^2 G(t)}{dt^2} = -\chi^2(t), \tag{S12}$$

where $G(t) = \frac{d^2\chi(t)}{dt^2}/\chi(t)$, and we have changed our notation from $\partial/\partial t$ to $d/dt$ because $\chi(t)$ is a function of time only. The cancellation of the $r_0$ dependence is due to the parabolic dependence of the thickness profile $d(r_0)$ on $r_0$,

thereby ensuring the linear dependence of the rhs of the Eq.(S11) on $r_0$. Therefore, Eq.(S12) defines the paraxial UC model for the non-relativistic case of $\Gamma \ll 1$.

The dependence of $\chi$ on $t$ is plotted in Fig. S2 (a) as the red curve, and the focal length solved from the UC model is $L_f \approx 2.5R_c$ instead of the more accurate $L_f \approx 2.95R_c$ calculated from the full DM model. This approach shows that the target motion in the sub-relativistic limit can also be described by a single contraction curve and it's essential to have a quadratic thickness profile to make this happening.

The discrepancy between the DM and UC models is due to the neglect of the finite angle $\alpha_i$, A more rigorous and accurate approach is to keep the $\cos^2\alpha_i$ term in Eq. (S8). The derivation for $\chi(t)$ is similar but lengthy. Therefore, only the resulting modified UC model equation is presented here:

$$\frac{d^2G(t)}{dt^2} = 4G^2(t) - \chi^2(t). \tag{S13}$$

In conclusion, we have numerically shown that for an arbitrary value of $\Gamma$, the target can always be focused into a small area. We also have found the formula for focal length $L_f \approx \left(2\Gamma^{1/2} + 2.95\right) R_c$ which is valid for arbitrary $\Gamma$. Further analytics have proven that, in both ultra-relativistic regime (case (i): $\Gamma \gg 1$) and sub-relativistic regime (case (ii): $\Gamma \ll 1$), the target can be described by a single contraction coefficient $\chi(t)$, that implies the target focusing is uniform and aberration-free. This derivation is valid only for a parabolic thickness distribution: the first-derivative of $d(r_0)$ must be linear to cancel the $r_0$ dependence in Eq. (S4) and Eq. (S10). Although the solutions of $\chi(t)$ show small discrepancies in both regimes, more rigorous derivations exist without neglecting terms in the equations of motion. Therefore, we conclude that, at least in these two limiting cases, the target can be focused into a point when its thickness is described by a parabolic function. Remarkably, this conclusion remains valid under more general conditions (arbitrary $\Gamma$) and has been confirmed by our numerous simulations using different $\Gamma$'s.

## II. OPTIMIZATION OF THE TARGET PARAMETERS

In all simulations in the main text, we have chosen the target thickness at its center point $d_0 = \eta_1 d_{\text{opt}}$, and $\eta_1$ is a number of order unity. Because the target thickness decreases towards the periphery of the target, we have additionally imposed a condition of $\eta_1 > 1$. The radius of the target was chosen to be comparable to its radius of curvature $R_c$: $R_0 = \eta_2 R_c$, where $\eta_2$ is a number of order unity. This restriction was made from practical consideration: if $\eta_2 \sim \sqrt{2}$ for the parabolic target thickness profile, then the target becomes very thin at its edge. On the other hand, if $\eta_2 \ll 1$, then the target is essentially planar, and the new physics associated with LILA cannot be captured. Therefore, for all simulations we have chosen $\eta_1 = 1.2$ and $\eta_2 = 1.14$. For these numerical values of $\eta_{1,2}$, the wave amplitude is estimated from the expression for the acceleration in terms of $a_0$ given by $g = 2\pi a_0(c^2/\lambda_L)(d_{\text{opt}}/d_0)(m_e/m_i)$, and from the definition of $\Gamma$ that can be expressed as $g = \Gamma c^2/R_c$. Combining these expressions and taking the value of $\eta_1$ into account result in the following expression for $a_0$: $a_0 = \Gamma(\lambda_L/R_c)(m_i/m_e)(d_0/d_{\text{opt}})/(2\pi) \approx 350\Gamma(\lambda_L/R_c)$. Inserting this expression of $a_0$ into a formula for the laser power incident upon a disk with the radius $R_0$, and taking into account the value of $\eta_2$, the following expression for the laser power $P_L$ is obtained: $P_L \approx 13.7 \times \Gamma^2\ PW$. By varying $\Gamma$, we have considered the targets with the radii $R_0$ as small as $R_0 = 2\lambda_L$ and as large as $R_0 = 10\lambda_L$. For the range of $\Gamma$'s tested in our simulations, the equivalent laser power varied between $P_L \approx 2.8$PW for $\Gamma \approx 0.45$ to $P_L \approx 35$ PW for $\Gamma = 1.61$ as listed in Table I of the main text. 3D-PIC simulation of the case corresponding to $P_L \approx 4.2$ PW is considered below.

## III. A MODERATE-POWER EXAMPLE: $P_L = 4.2$PW AND AN ALL-HYDROGEN LILA TARGET

This section presents an example of a laser-target configuration that can be achievable using present-day laser systems[1]. Recently unveiled petawatt laser facilities can already generate a $P_L = 4.2$PW, $\tau_L = 20$fs laser pulse[1]. Several 10PW-scale laser facilities are under construction [2, 3]. We have mentioned in the main text that 3D PIC simulations of the LILA targets have been carried out by us. Target have been found to be stable for a wide range of laser powers: 2.8PW $< P_L <$ 35PW. Here we present one specific example of a small all-hydrogen variable-thickness target illuminated by a laser pulse with a peak power of $P_L = 4.2$PW. Extensive details of our numerical model are also presented below.

A 3D PIC simulation was carried out using the relativistic electromagnetic code VLPL [4]. The computational domain of the size $X \times Y \times Z = 20\lambda_L \times 10\lambda_L \times 10\lambda_L$, where $\lambda_L$ is the laser wavelength, consists of $2000 \times 125 \times 125$ grid cells. Each cell contains 160 macro-particles emulating electrons and hydrogen ions. The LILA target with maximum thickness $d_0 = 350nm$, radius of curvature $R_c = 2.1\lambda$ and radius $R_0 = 2.4\lambda$ is initially placed at $X = 5\lambda$. The initial proton density is $n_0 = 100n_c$. A $25fs$ circularly-polarized laser pulse is incident from the left boundary

and has a flat-top profile in both transverse and longitudinal directions. The normalized vector potential $a_0 = 92$ and wavelength $\lambda_L = 1\mu m$, corresponds to the power $P_L = 4.2$PW on the target.

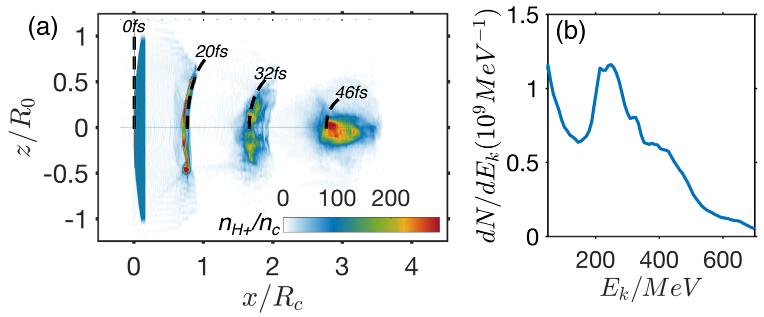


FIG. S3: A 3D PIC simulation of LILA with $P_L = 4.2$ PW incident laser power. (a) Snapshots of ion densities. Black-dashed lines: predicted target position from the DM model. The focal spot (peak plasma density) is achieved at $t_f = 46fs$. (b) Proton kinetic energy spectrum at $t = t_f$.

Fig. S3 (a) shows the overlaid time snapshots of proton density $n_{H^+}$ in the $x-z$ cross-section. On top of that, we also plotted the results(black dashed line) from the Deformable Mirror(DM) model and they agree with each other quite well. The target reaches the focal point at the time $t_f = 46$fs corresponding to the focal distance $L_f \sim 3R_c \approx 6.3\mu m$. Approximately 33% of all target protons are focused into the hot spot, where the proton density reaches $n_{\max} \approx 200n_c$ which is twice the initial density. Fig. S3 (b) shows the kinetic energy spectrum of all protons at $t = t_f$. While not truly mono-energetic at this laser power, the spectrum does exhibit a clear peak at $E_k \approx 250$MeV.

## IV. LILA USING A GAUSSIAN LASER PULSE

This section addresses the feasibility of LILA driven by a laser pulse with a realistic (Gaussian) transverse profile: $I = I_0 \exp(-r^2/\sigma_L^2)$, where $\sigma_L$ is the spot size of the laser. To focus/accelerate a variable-thickness target by such a laser pulse, an appropriate correction must be applied on the optimal target thickness $d(r_0) \to d(r_0)\exp(-r^2/\sigma_L^2)$. This correction accounts for the radial dependence of the radiation pressure. Using a 3D simulation below, we show that this redesigned all-hydrogen target indeed performs in the same as a parabolic-density target accelerated by a planar laser pulse. In this simulation, the computational box size is chosen to be $X \times Y \times Z = 50\lambda_L \times 20\lambda_L \times 20\lambda_L$. It consists of $5,000 \times 250 \times 250$ grid cells. Each cell contains 160 macro-particles. The LILA target is initially place at $X = 5\lambda$; its thickness is $d_0 = 300nm$, the radius of curvature is $R_c = 7\lambda$, and the total radius is $R_0 = 8\lambda$. The initial proton density is $n_0 = 150n_c$(we increased the density to compensate for the decrease of thickness due to the applied correction, however, one can choose to increase the thickness instead). A $\tau_L = 46$fs circularly-polarized laser pulse is incident from the left boundary. It is assumed to have a flat-top longitudinal profile and a Gaussian transverse profile with a spot size $\sigma_L = R_0 = 8\lambda$. The peak normalized vector potential of the laser is $a_0 = 80$, corresponding to $P_L = 35$PW on the target.

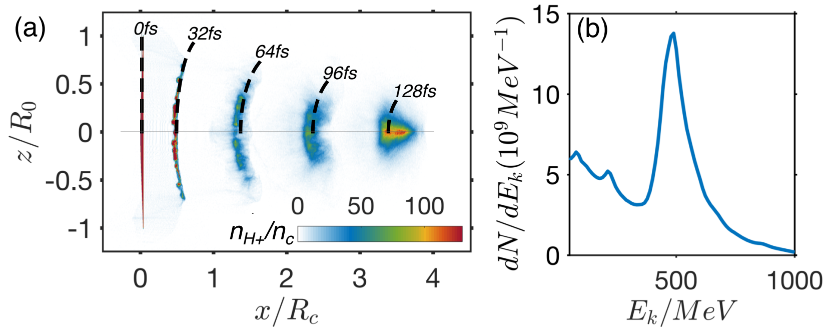


FIG. S4: A 3D PIC simulation of LILA of a variable-thickness target by a transversely Gaussian laser pulse. The target thickness is adjusted by the laser profile. (a) Snapshots of ion densities. Black-dashed lines: target position according to the DM model. The focal spot (peak plasma density) is reached by the target at $t_f = 128$fs. (b) Proton kinetic energy spectrum at $t = t_f$.

Fig. S4 (a) shows the overlaid time snapshots of proton density $n_{H^+}$ in X-Z cross-section, and the black dashed lines represent the results predicted by the DM model. The target is focused at $t_f = 128$fs, corresponding to the focal length $L_f \sim 3.5R_c \approx 24.5\mu$m. Approximately 45% of all target protons are focused into the hot spot at the focal point, and its density reaches $100n_c$. Fig.S4 (b) shows the kinetic energy spectrum of all protons at $t = t_f$. A quasi-monoenergetic proton beam with $E_k \approx 500MeV$ converges onto the focal point.

## V. AN EXAMPLE OF A TWO-ION-SPECIES LILA TARGET

This section addresses the viability of the LILA concept when applied to a realistic (multi-ion species) target. Here we assume a hydrocarbon target with two ion species: fully-ionized carbons ($C^{+6}$) and protons that are neutralized by electrons. Acceleration of multi-ion plasmas in the RPA regime has been extensively discussed[5–7], but only in the context of flat (constant-thickness) targets. Due to the difference of the $Z_j/m_j$ (where $Z_j$ and $m_j$ are the $j$'th ion species charge state and mass, respectively) ratio between a proton and carbon, a two-layer structure develops during the acceleration [6, 7]. In principle, the heavier (smaller $Z/m$) ions can travel together with the protons after a fast separation phase during the early acceleration stage. Therefore, the target can be still regarded as a monolithic charge-neutral plasma despite the details of its composition. The DM model should still work for the LILA design, but the peak energy $\Gamma$, which defines the acceleration of the target, should be modified to account for the change in charge/mass ratio: for the same laser parameter and electron density, the $\Gamma[CH] \rightarrow \frac{Z_H+Z_C}{A_H+A_C}\Gamma[H] = \frac{7}{13}\Gamma[H]$, where $Z_j$ is the ion charge state and $A_j$ is the atomic mass number.

We have carried out a 3D PIC simulation of a C-H target using the following computational domain parameters: the domain size is $X \times Y \times Z = 40\lambda_L \times 14\lambda_L \times 14\lambda_L$, the grid size is $6,666 \times 175 \times 175$ cells, and each cell contains 200 macro-particles. The carbon-proton LILA target with the maximum thickness $d_0 = 210$nm, the radius of curvature $R_c = 4.5\lambda_L$, and the total radius $R_0 = 5.1\lambda_L$ is initially placed at $X = 5\lambda_L$ . We use pre-ionized plasma with equal number of $C^{6+}$ and $H^+$ particles. The electron density is $200n_c$ and the proton/carbon ion density is $28.57n_c$. A $\tau_L = 32$fs circularly-polarized laser pulse with a flat-top transverse/longitudinal profile is incident from the left. The normalized vector potential of the laser pulse is $a_0 = 110$, corresponding to the power of $P_L = 21$PW on the target.

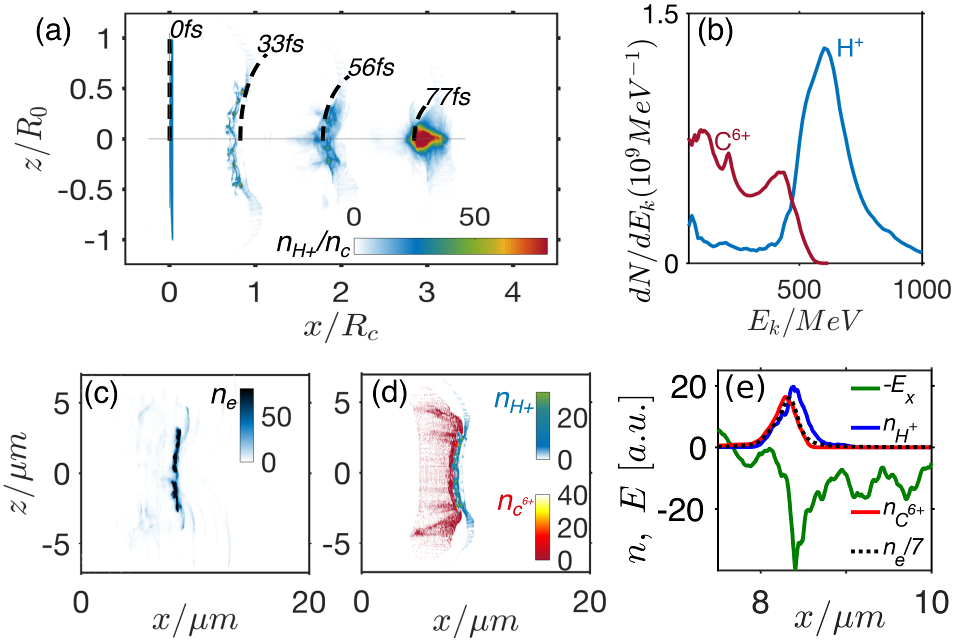


FIG. S5: A 3D PIC simulation of the LILA utilizing a C-H target. (a) Snapshots of the ion densities. Black-dashed lines: target position estimated from the DM model. The focal spot (peak plasma density) is achieved at the time $t_f = 77fs$ (b) Ion energy spectrum at $t = t_f$. (c) Electron density at $t = 33fs$. (d) A two-layer structure formed by protons and carbons at $t = 33fs$. (e) One-dimensional distributions of electron density, ion densities and longitudinal electric field.

Fig. S5 (a) shows the overlaid time snapshots of proton density $n_{H^+}$ in X-Z cross-section. There is a good agreement between the PIC simulation results and the predictions of the DM model(black dashed lines). The target is focused at $t_f = 77$fs corresponding to the focal length of $L_f \sim 3R_c \approx 13.5\mu$m. Approximately 70% of the protons contained in the target are focused into the hot spot at the focal point, where the proton density reaches $80n_c$ (i.e. almost

three times the original proton density). On the other hand, only $\approx 25\%$ of carbon ions are focused at the focal point. The percentage of focused protons is much higher compared to those of all-hydrogen targets ($\approx 50\%$). In an all-hydrogen target, it's known that a considerable fraction of the protons is left behind in the ion tail [8]. However, in a two-ion-species target, the "light" protons are accelerated faster than the "heavier" carbon ions. Even after the heavier (lower $Z/m$ ratio) ions catch up and produce a two-layer structure, the protons are effectively "pushed" by the heavier ions from behind because the latter provide electrons that run ahead of the protons. Therefore, more protons can be accelerated and focused into the focal spot. One can also observe in Fig. S5 (a) that the proton density shows some signs of the RT-like instability at $t = 33$fs, which is also observed in Fig. 3 (a) in the main text. However, this instability is effectively suppressed due to the convergence of the accelerated target. The existence of the heavier ions can also mitigate the RT-like instability, as pointed out by [6, 7]. Figure S5 (b) shows the kinetic energy spectrum (per nucleon) of all protons and carbon ions at $t = t_f$. A quasi-monoenergetic peak of accelerated protons is observed at $E_k \approx 600$MeV. The $E_k$ per nucleon of $C^{6+}$ is smaller than protons, but their velocities are not very different from those of the protons: the average longitudinal velocity of $C^{6+}$ near the focal spot is $\sim 90\%$ of the longitudinal velocity of protons. Figure S5 (c-e) show the acceleration details at $t = 33$fs. The bending of the entire target is observed in Fig. S5 (d), where we can also observe the formation of a two-layer-structure comprised of $H^+$ and $C^{6+}$ ions. The light proton (blue-green) beam is moving slightly ahead of the heavier carbon (red) ion beam, and more carbon ions are left behind.


[1] J. H. Sung, H. W. Lee, J. Y. Yoo, J. W. Yoon, C. W. Lee, J. M. Yang, Y. J. Son, Y. H. Jang, S. K. Lee, and C. H. Nam, "4.2 PW, 20 fs Ti: sapphire laser at 0.1 Hz," *Opt. Lett.* vol 42, 11 (2017).

[2] W. Li, Z. Gan, L. Yu, C. Wang, Y. Liu, Z. Guo, L. Xu, M. Xu, Y. Hang, Y. Xu, J. Wang, P. Huang, H. Cao, B. Yao, X. Zhang, L. Chen, Y. Tang, S. Li, X. Liu, S. Li, M. He, D. Yin, X. Liang, Y. Leng, R. Li, and Z. Xu, "339 J high-energy Ti: sapphire chirped-pulse amplifier for 10 PW laser facility," *Opt, Lett.* vol 43, 22 (2018).

[3] B. Le Garrec, D. N. Papadopoulos, C. Le Blanc, J. P. Zou, G. Chériaux, P. Georges, F. Druon, L. Martin, L. Fréneaux, A. Beluze, N. Lebas; F. Mathieu, P. Audebert, "Design update and recent results of the Apollon 10 PW facility," *Proc. SPIE* vol 10238, 80 (2017).

[4] A. Pukhov, "Three-dimensional Electromagnetic Relativistic Particle-in-cell Code VLPL (Virtual Laser Plasma Lab)," *J. Plasma Phys.* vol 61, 425 (1999).

[5] A. P. L. Robinson, M. Zepf, S. Kar, R. G. Evans, and C. Bellei, "Radiation pressure acceleration of thin foils with circularly polarized laser pulses," *New J. of Phys.* vol 10, 1 (2008).

[6] T. P. Yu, A. Pukhov, G. Shvets, and M. Chen. "Stable laser-driven proton beam acceleration from a two-ion-species ultrathin foil," *Phys. Rev. Lett.* vol. 105, 6 (2010).

[7] T. P. Yu, A. Pukhov, G. Shvets, M. Chen, T. H. Ratliff, S. A. Yi, and V. Khudik. "Simulations of stable compact proton beam acceleration from a two-ion-species ultrathin foil," *Phys. Rev. Lett.* vol 18, 4 (2011).

[8] V. Khudik, S. Yi, C. Siemon, and G. Shvets, "The Analytic Model of a Laser-accelerated Plasma Target and Its Stability," *Phys. Plasmas*, vol 21, 013110 (2014).
